# Supplementary material for: Adaptive VIO: Deep Visual-Inertial Odometry with Online Continual Learning
Source: arXiv:2405.16754 source file (2024-05-27)
Supplement: Supplementary file 1 [file X_suppl.tex]

\clearpage
\setcounter{page}{1}
\maketitlesupplementary

\section{Additional Details on the VIO System}
\label{sec:system}
The main components of Adaptive VIO are illustrated in Fig.\ref{system}, which can be divided into four modules: prediction, optimization, feedback, and keyframing. Prediction and optimization (except for initialization) are collectively called tracking in this paper.

As an extension to Sec.\ref{subsec: online}, we provide additional technical details about the VIO system in the following content.

\textbf{Initialization:} We use 8 frames for map initialization, where the procedure is the same as DPVO\cite{dpvo}. To achieve higher initialization accuracy, we require sufficient parallax between frames. As for IMU initialization, we conduct the Maximum-a-Posteriori estimation as ORB-SLAM3\cite{orbslam3} does. The states for initialization include velocity, scale, gravity direction, and IMU bias. We perform IMU initialization twice when accumulating 40 frames and 80 frames, respectively. Between map initialization and IMU initialization, we run visual bundle adjustment to track each frame. All frames are treated as keyframes, and keyframe culling is not performed. After IMU initialization, we obtain the initial values for states with metric scale and aligned coordinates, then the system enters the tracking process.

\textbf{Tracking:} For each incoming frame, we sample 96 feature patches and search for their correspondences with the previous 13 keyframes. The initial pose estimation of the new frame is generated by the IMU motion model. As for optimization, the states of the latest 10 keyframes in the factor graph are subject to optimization, while the states of other frames are fixed. Considering efficiency, during online continual learning, only the last 4 frames have IMU constraints, while in the formal deployment, all keyframes within the sliding window have IMU constraints. We perform 2 iterations of VIBA for each tracking.

\textbf{Feedback:} During online continual learning, after each tracking procedure, feedback losses are backpropagated to the visual correspondence predictor and IMU bias predictor. Considering resource and time consumption, not all constraints in the factor graph are used as error terms. We found that the loss calculated for IMU and vision is large for the most recent few frames, while the loss between previous keyframes is very small. Hence, for the IMU network, we construct preintegration loss for the last 2 frames. For the visual network, we constitute the photometric loss for the feature patches from the last 4 frames. The feature patches are reprojected into all associated keyframes in the factor graph. Besides, due to partial overlap between keyframes, patches in the projected positions of the target image that extend beyond the image boundaries are excluded from loss calculation.

\begin{figure}[t]
  \centering
  \includegraphics[width=0.48\textwidth]{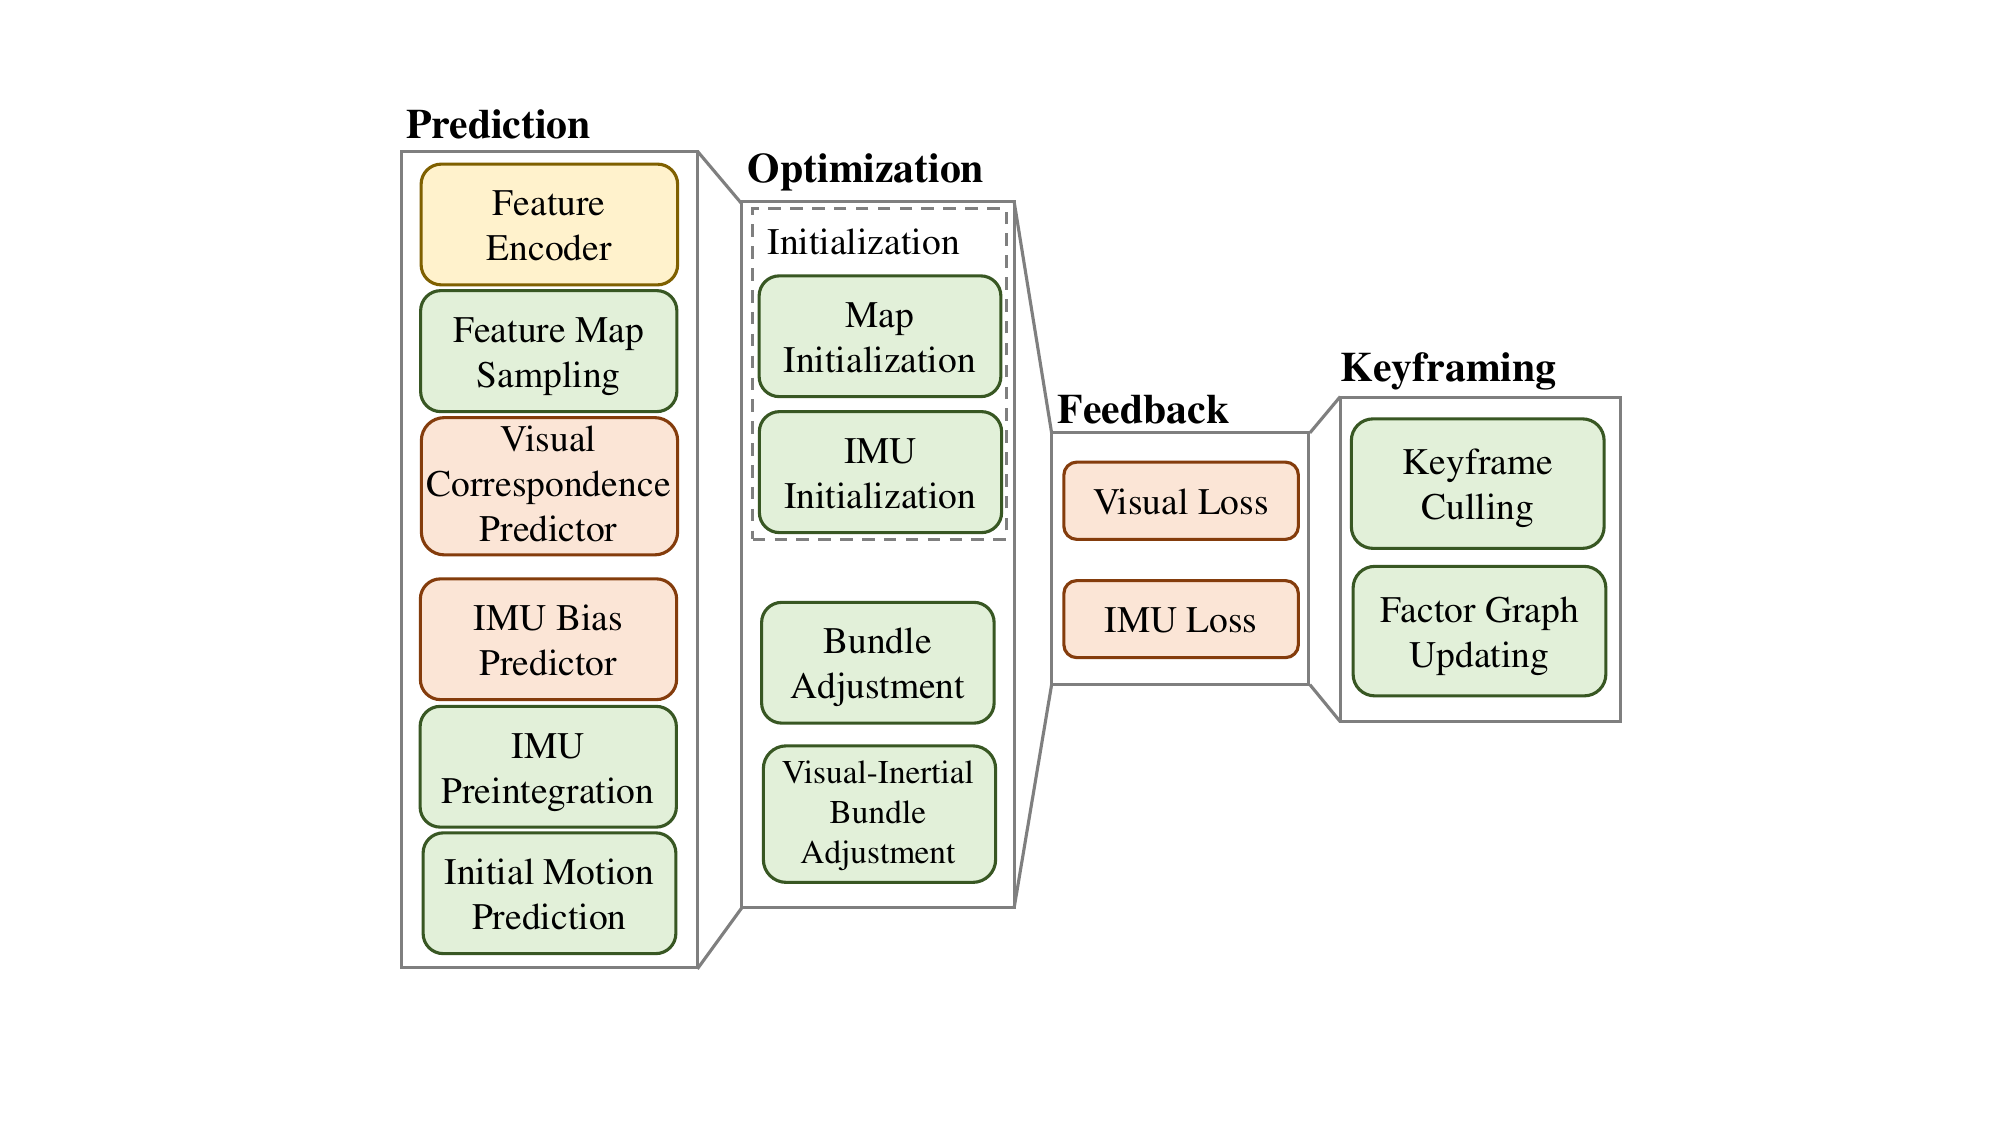}
  \caption{Main system components of Adaptive VIO. Learning-based modules are colored in yellow and orange. Traditional computational modules are colored in green.}
  \label{system}
\end{figure}

\textbf{Keyframing:} The keyframing strategies include keyframe culling and factor graph updating. For each input frame, we temporarily consider it as a keyframe. However, when it becomes the fourth-to-last ($t-4$) frame, we reassess whether to retain it as a keyframe. During online continual learning, we verify if the disparity between keyframes $t-5$ and $t-3$ is sufficient. If it is, we retain the $t-4$ frame; otherwise, we remove the frame from the keyframe sequence and eliminate all related constraints in the factor graph. In the formal deployment, we additionally require that after removing two consecutive keyframes, the next keyframe must be retained. This is to ensure the stability of IMU constraints within the sliding window. Besides, as for the formal deployment, when a keyframe is retained, we also construct a covisibility graph for it. Except for the keyframes already associated with it, we calculate the disparity between this frame and other keyframes. If the disparity is less than the median disparity of the already associated keyframes, we establish a covisibility relationship between the two keyframes. For efficiency, the number of such covisibility relationships should not exceed 8 pairs. Then we add these new visual constraints to the factor graph.

We may notice the differences in the system settings between online continual learning and formal deployment. This is primarily due to two reasons. 1) Online learning requires more computational resources and time because of the need to compute feedback loss and perform backpropagation. In order to get real-time or near real-time processing for both settings, the factor graph is simplified compared to the formal deployment. 2) Although factor graphs with covisibility relationships offer higher accuracy, they attenuate the weights of correspondences with large errors, which may be counterproductive for network learning.

Our system demands around 16GB of GPU memory during online continual learning and 12GB during formal deployment.

\begin{figure}[t]
  \centering
  \includegraphics[width=0.48\textwidth]{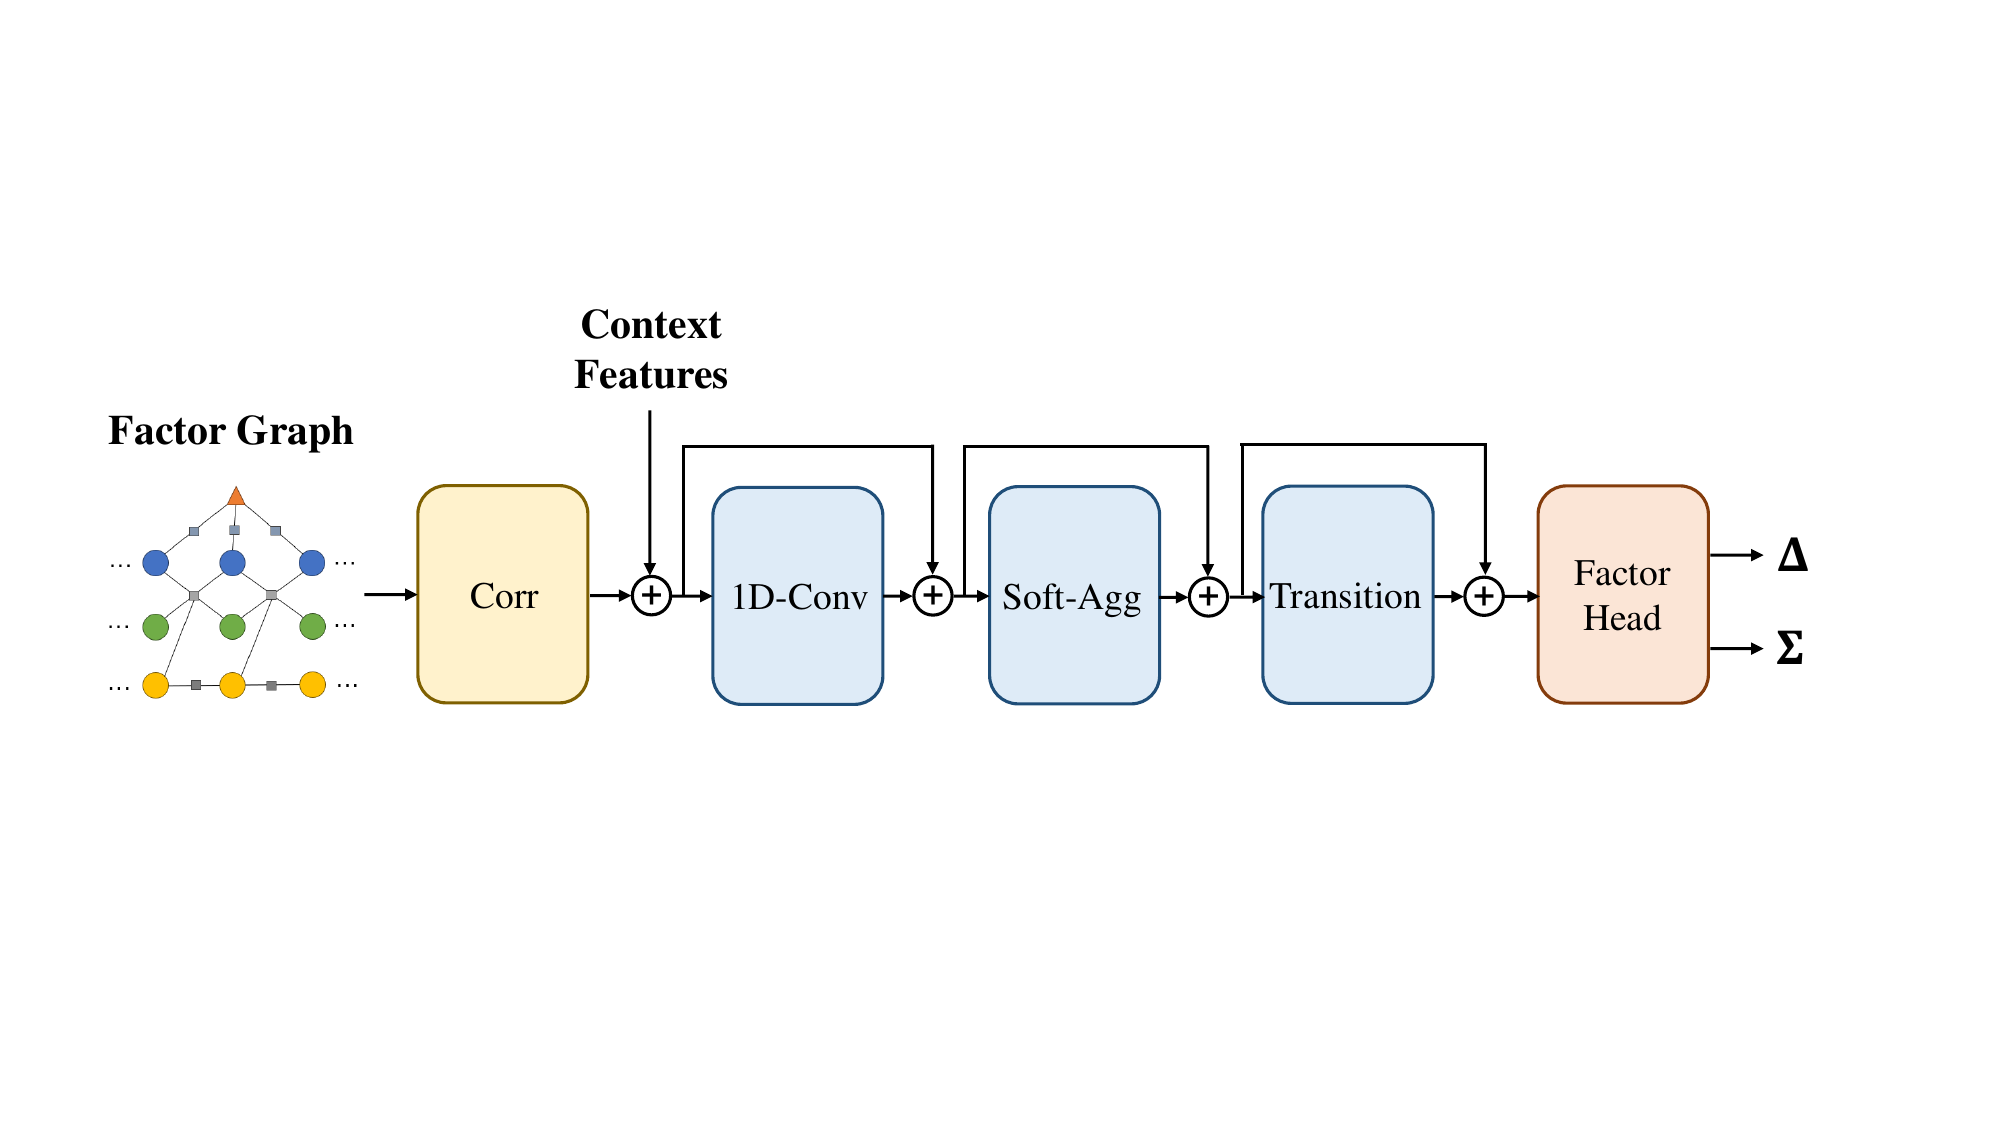}
  \caption{Network Architecture of Visual Correspondence Predictor.}
  \label{visualnet}
\end{figure}

\begin{figure}[t]
  \centering
  \includegraphics[width=0.48\textwidth]{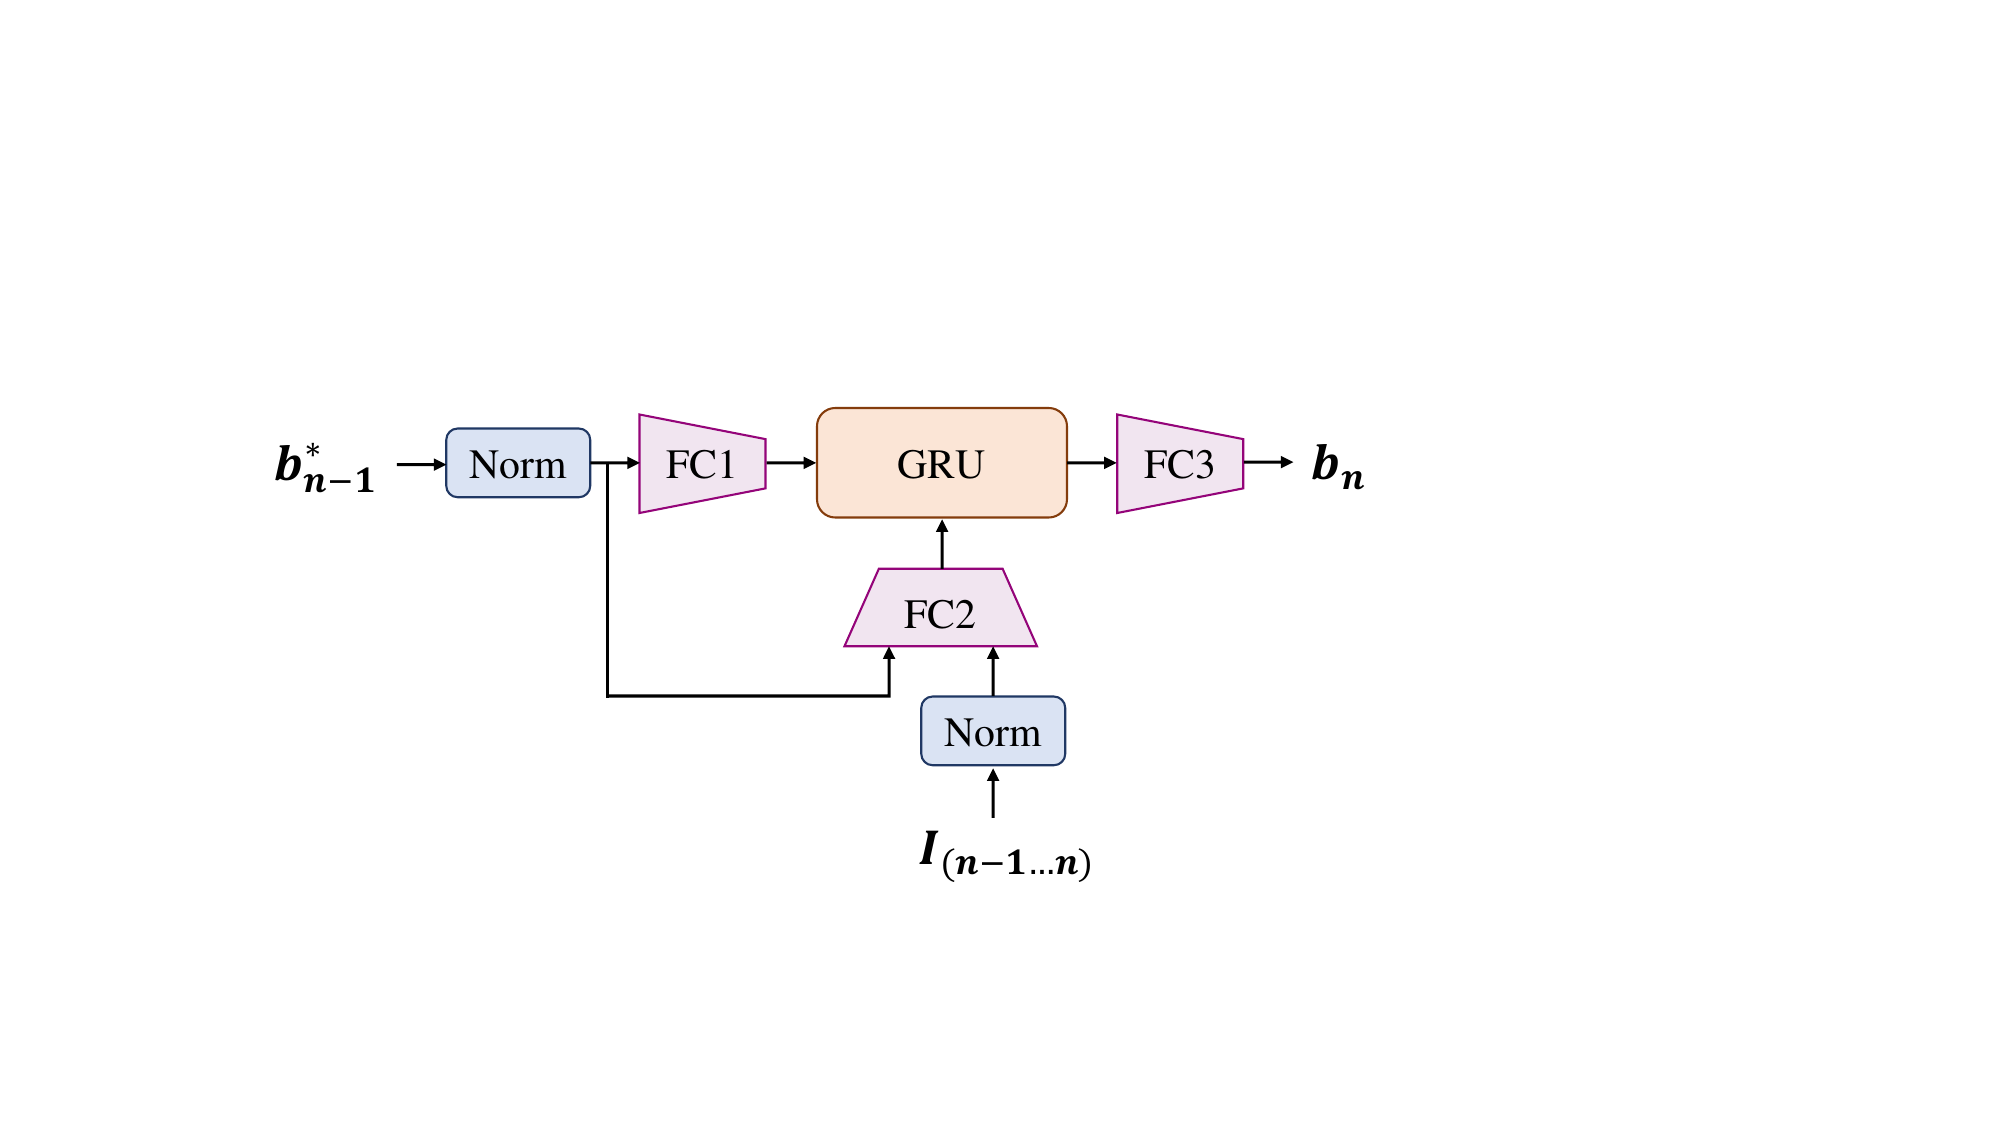}
  \caption{Network Architecture of IMU Bias Predictor.}
  \label{biasnet}
\end{figure}

\section{Network Architecture}
\label{sec:network}
In this section, we present the network architecture of our visual and IMU networks.

The paradigm of visual correspondence predictor is shown as Fig.\ref{visualnet}. The inputs of the network are the coordinates on the target frame after reprojection, along with the context features of the target frame. After passing through the correlation layer and other network layers, the factor head outputs the predicted correspondence updates (residuals) and their weights. A detailed description of each component can be found in DPVO, where the network is referred to as the "update operator".

Please note that, unlike the update operator in DPVO, our visual correspondence predictor does not contain a hidden state. The hidden state plays a role in conveying information during multiple calls to the network. Since our online continual learning conducts backpropagation after each tracking iteration, canceling the hidden state can alleviate the mutual influence between multiple iterations, making every prediction an independent procedure. This design makes online adaptation more efficient and robust.

The architecture of the IMU bias predictor is shown in Fig.\ref{biasnet}. $\mathbf{b^*_{n-1}}$ is the optimized bias estimates for the previous frame, and $\mathbf{b_n}$ is the bias prediction for the current frame. $\mathbf{I_{n-1...n}}$ represents the IMU measurements in between. The inputs are first normalized and then fed into fully connected layers (FC1, FC2). FC1 encodes the bias as the initial hidden state for the GRU, while FC2 encodes the concatenation of bias and measurements as the input of the GRU. The final hidden state from the GRU is restored to the current bias prediction through the FC3 layer. The hidden size for the GRU is set to 64 in our method. The network models the inherent bias variations of the sensor. Compared to the random walk model, it mitigates the continuous propagation of sudden bias estimation errors over time, making the system more stable.

The bias predicted by the network originates from two aspects. 1). For low-cost MEMS IMU, the bias in its static state is referred to as fixed bias. It is inherent to the sensor and associated with errors during manufacturing. This bias remains approximately constant and cannot be entirely eliminated by factory calibration. 2). With the motion of the agent, the IMU bias is also influenced by both acceleration and angular velocity, especially in scenarios with rapid changes in motion. The classic methods rely on extrinsic parameter calibration to estimate fixed bias, whereas our approach replaces it with neural networks. Additionally, the networks also consider the influence of motion on bias variation, thereby enhancing the accuracy and robustness of the system.

We may notice that the inputs of both visual and IMU networks are from the previous optimization, and the outputs of both networks are served for the subsequent optimization. Such a pipeline where learning and computation mutually support each other is a distinctive feature of our VIO system.

% \section{GPU Acceleration and Running Speed}
% \label{sec:runtime}

% Unlike classic VIO systems running on the CPU, most data and processing in our approach are conducted on the GPU. 

% In practice, we leverage the advantages of GPU to accelerate computations. For IMU processing, batch computations are employed to accelerate the IMU preintegration, along with the residual and Jacobian calculations during optimization. For visual processing, in formal deployment, we utilize C++ and CUDA extension of PyTorch to further accelerate the computation of residuals, Jacobians, and Hessians. However, during online continual learning, as loss functions require backpropagation through the factor graph, the process is still implemented in Python. Our system demands around 16GB of GPU memory during online continual learning and 12GB during formal deployment.

% Thanks to the GPU acceleration, our method achieves a frame rate of 26FPS during formal deployment, which is real-time for common datasets with 20Hz cameras. While during online continual learning, the average frame rate is approximately 20FPS. This is due to the additional computation time introduced by feedback, including loss computation and backpropagation. Although reducing the number of features and frames can further enhance the real-time performance of online continual learning, it implies poorer tracking accuracy and a longer adaptation time, which is a trade-off. Balancing real-time performance and tracking accuracy, achieving life-long continual learning and fast adaptation are the key focus for our future work.

\section{Implementation of Optimization}
\label{sec:runtime}
Unlike classic VIO systems running on the CPU, most data and processing in our approach are conducted on the GPU. 

We leverage the advantage of GPU batch processing to accelerate IMU processing, including computing preintegration, covariance, Jacobian, and Hessian matrices. For visual processing, in formal deployment, we utilize C++ and CUDA extension of PyTorch to further accelerate the computation of residuals, Jacobians, and Hessians. However, during online continual learning, as loss functions require backpropagation through the factor graph, the process is still implemented in Python. 

For visual-inertial bundle adjustment, we combine the IMU and visual counterparts with equal weights and utilize the Gauss-Newton method for optimization. Like VI-DSO and DM-VIO, we also apply the Schur complement trick for matrix solving.
